# Supplementary material for: RENs: Relevance Encoding Networks
Source: arXiv:2205.13061 source file (2022-07-17)
Supplement: Supplementary file 2 [file appendix_image_results.tex]

\clearpage
\subsection{Image Results}\label{appendix_image_results}

\begin{figure}[ht]
    \centering
    \includegraphics[scale=0.8]{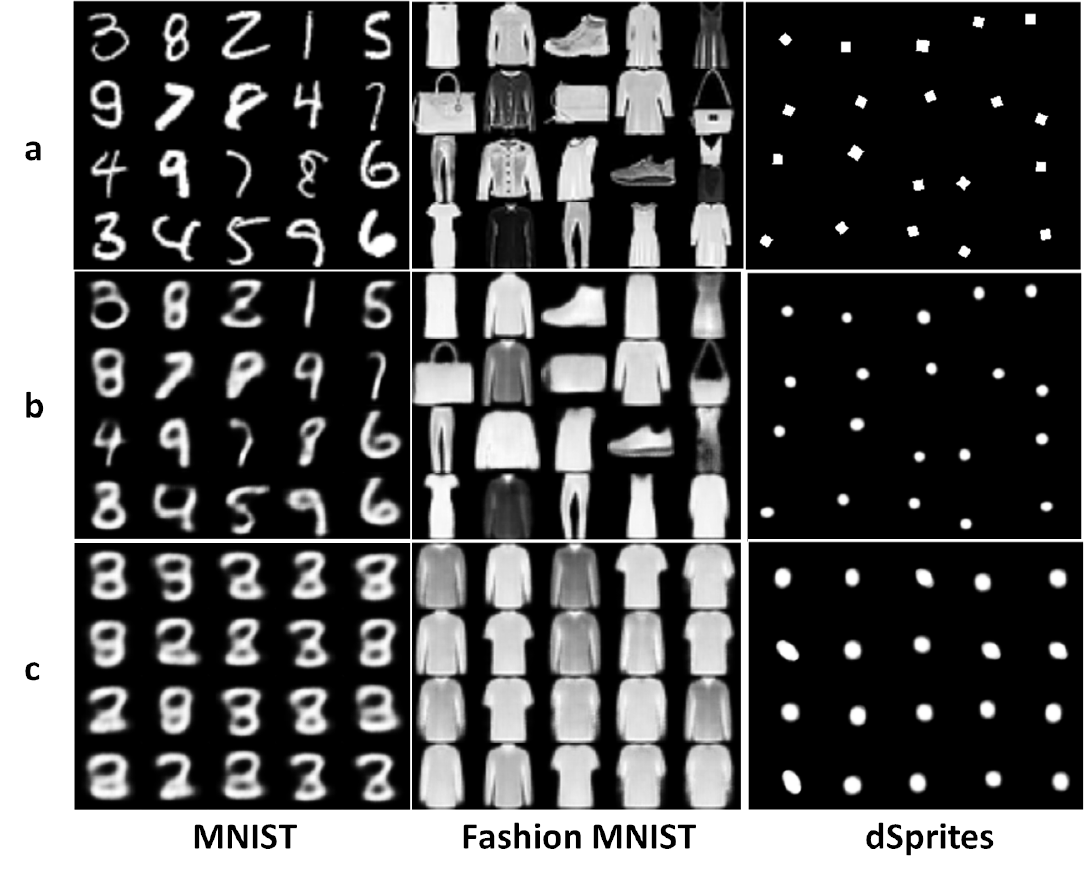}
    \caption{RF-VAE results of the best performing models from Table.\ref{tab_fid_gen}. We show (We show (a) original images, (b) reconstructed images, and (c) randomly generated images (no cherry-picking). (1) RF-VAE 32 for MNIST, (2) RF-VAE 32 for Fashion MNIST, (3) RF-VAE 10 for dSprites\\ \\}
    \label{fig:rfvae_best_model_images}
\end{figure}

\begin{figure}[ht]
    \centering
    \includegraphics[scale=0.8]{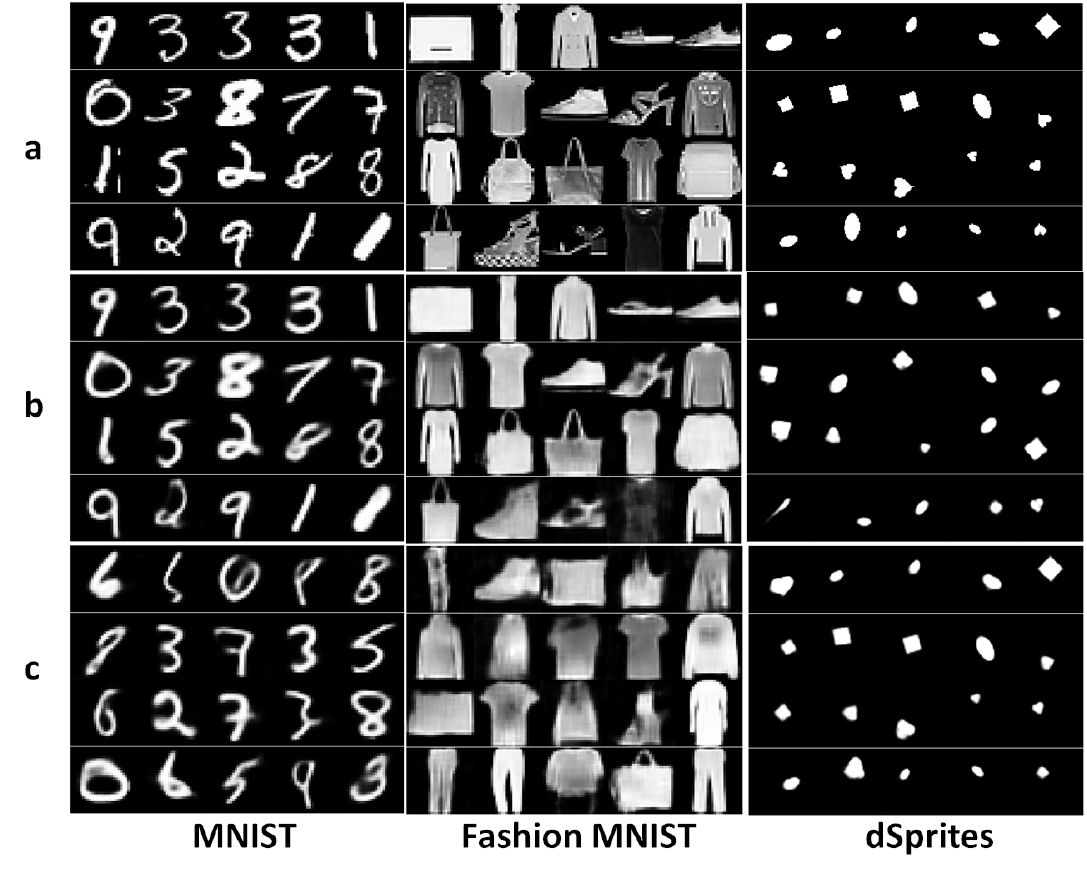}
    \caption{GECO results of the best performing models from Table.\ref{tab_fid_gen}. We show We show (a) original images, (b) reconstructed images, and (c) randomly generated images (no cherry-picking). (1) GECO 16 for MNIST, (2) GECO 64 for Fashion MNIST, (3) GECO 15 for dSprites\\ \\}
    \label{fig:geco_best_model_images}
\end{figure}

\begin{figure}[ht]
    \centering
    \includegraphics[scale=0.8]{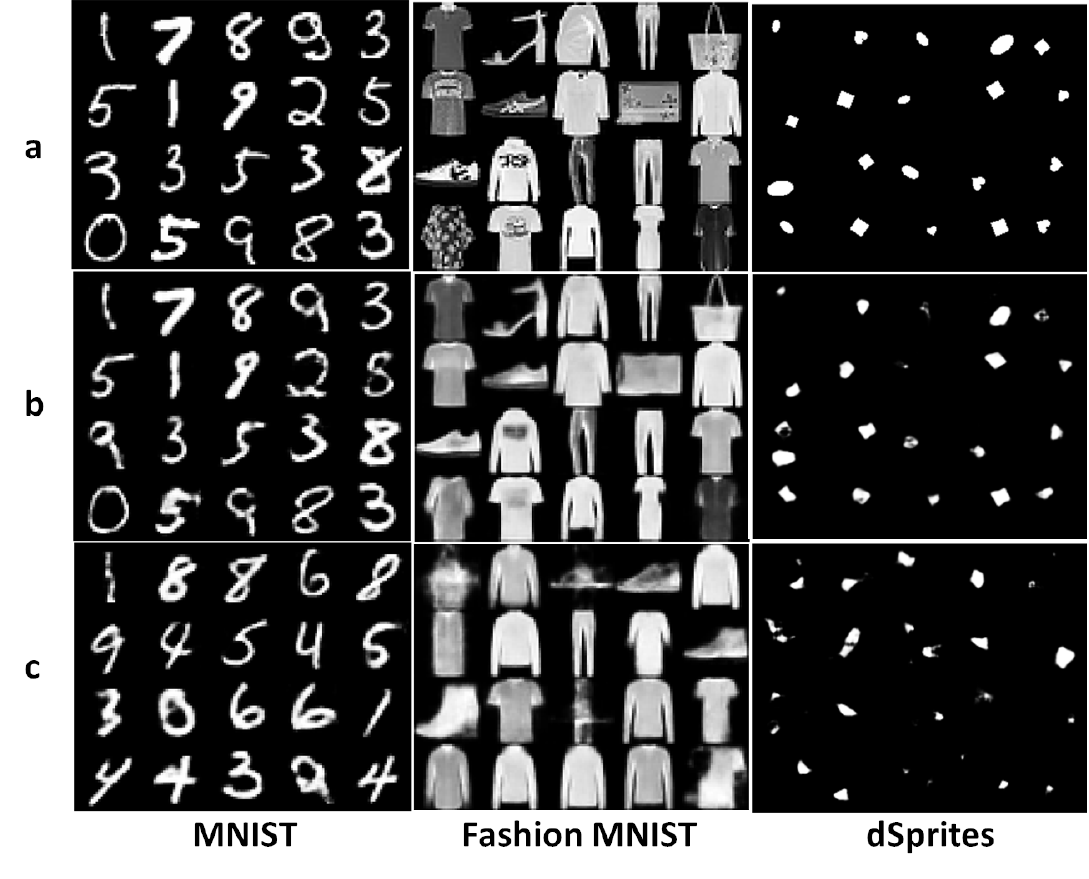}
    \caption{MAAE results of the best performing models from Table.\ref{tab_fid_gen}. We show We show (a) original images, (b) reconstructed images, and (c) randomly generated images (no cherry-picking). (1) MAAE 32 for MNIST, (2) MAAE 64 for Fashion MNIST, (3) MAAE 15 for dSprites\\ \\}
    \label{fig:maae_best_model_images}
\end{figure}
